# Supplementary material for: Annotation-efficient cancer detection with report-guided lesion annotation for deep learning-based prostate cancer detection in bpMRI
Source: arXiv:2112.05151 source file (2022-02-19)
Supplement: Supplementary file 2 [file thesis-appendices.tex]

\newpage
\appendix
\subsection{Rician noise}
% introduce data augmentations
Data augmentation is one of the most import techniques to improve the generalisation of deep learning models to unseen data. Typical data augmentations include rotation, mirroring, translation and zooming, but many more exist. When training a network with data augmentations, the training samples are transformed with one or multiple augmentations before being provided to the network. As a result, the network is guided to make its predictions invariant under these transformations, which results in a model that generalises better to unseen data. 

% introduce intensity based augmentations
At the start of my internship, the group's data augmentation pipeline consisted of rotation, translation, horizontal flipping and zooming, which are all geometric transformations. To improve the data augmentation pipeline, I have investigated intensity based augmentations, which are complementary to geometric transformations. While geometric transformations move the original voxels around in some structured way, intensity based augmentations preserve the location of the voxels and apply noise to each voxel. 

% introduce Rician noise
Intensity based augmentations span a large domain of additive, multiplicative and/or any nonlinear function based on the original voxel value. %  and/or multiplicative noise, with noise parameters drawn from any distribution. 
One of the best known intensity based augmentations is additive Gaussian noise, where noise following the Gaussian distribution is added to each voxel individually:
\begin{equation}
    I_{new} = I_{old} + \mathcal{N}(0, \sigma^2)
\end{equation}
Where $\mathcal{N}$ is the Gaussian distribution and $\sigma^2$ the variance. 

A drawback of additive Gaussian noise is that the intensities can become negative, which is physically impossible for MRI sequences such as T2W and DWI (these scans as used by radiologists and this work are magnitude maps; phase maps can be negative, but are typically disregarded). Noise in MRI scans is shown to be governed by the Rician distribution \citep{gudbjartsson1995rician}, which is non-negative and approaches the Gaussian distribution for large values. The Rician distribution is given by:
\begin{equation}
    I_{new} = \sqrt{(I_{old} + \sigma \cdot \phi)^2 + (\sigma\cdot\phi)2}
\end{equation}
Where $\sigma$ is the magnitude of the Rician distribution and $\phi$ is drawn from $\mathcal{N}(0, 1)$ for each voxel individually.

\newcommand\footnoteMisalignment{\footnote{Accounting for the misalignment proved difficult, so I excluded \numVisitsMisalignedExcluded\ cases ($1.6\%$) which otherwise would have a misalignment of at least 2 mm. }}

% introduce dynamic preprocessing pipeline
Motivated by the physical relevance of the Rician distribution, I have adapted the data pipeline to incorporate this distribution as data augmentation. This required an overhaul of the way the scans are preprocessed, because the Rician noise needs to be applied at native resolution and initially the scans were resampled at an early stage. The new preprocessing pipeline saves the scans at original resolution, and resamples them on-the-fly during model training, after applying the Rician noise data augmentation. This overhaul also resulted in a good understanding of the preprocessing steps, which led to the discovery of a bug where T2W and ADC/DWI scans became misaligned due to the preprocessing pipeline\footnoteMisalignment.

% introduce experiment
To determine a good magnitude for the Rician noise ($\sigma$), I identified the range of $\sigma \in [0, 0.05]$ as relevant values through visual inspection, and tested $\sigma=0.00$, $0.01$, $0.02$, $0.03$, $0.04$ and $0.05$. During training, the Rician noise is applied with a probability of $75\%$. For each magnitude, models were trained with 5-fold cross-validation and 2 restarts. The resulting 10 performance metrics were compared using the permutation test with \numIterationsPermutationTest\ iterations. To retain the integrity of the external test set (ZGT), each model is evaluated on the RUMC dataset. 

% results
To evaluate the patient based diagnostic performance we can leverage the \numUnlabelledStudiesFullDataset\ unlabelled RUMC visits, which results in a much more stable evaluation compared to the $\approx 300$ labelled studies in each validation fold\footnote{This number is lower than 1/5th of all labelled samples, because samples with positive MRI (PI-RADS $\geq 3$) but unknown biopsy result were excluded from the validation set. }. For these unlabelled visits the ground truth is derived by automatically extracting the scores from pathology and radiology reports. To construct labels with low error rate and typical distribution of low-, intermediate and high risk patients, a method similar to ProstateX was employed: cases with Gleason grade group $\geq 2$ are positive and cases with either Gleason grade group $\leq 1$ or PI-RADS $\leq 2$ are negative. This gives 883 biopsy-confirmed positive cases and 2,656 negative cases. 

The patient based diagnostic performances as evaluated against the ProstateX-like labels are given in \Cref{fig:rician-noise-AUC-performance}. The statistical significance p-values are given in \Cref{fig:rician-noise-AUC-significance-matrix}. Small amounts of Rician noise ($\sigma \in [0.01, 0.03]$) as data augmentation may improve patient based model performance, but not with statistical significance ($P = 0.17-0.55$). 
\input{figures/rician-noise-AUC-performance}
\input{figures/rician-noise-AUC-significance-matrix}

To evaluate lesion based diagnostic performance, manually annotated cases are required. The 5-fold cross-validation results in five validation sets with small differences in difficulty, resulting is slightly higher or lower performance metrics across all models for some validation folds. Differences in model performance can be highlighted by accounting for this variation intrinsic to the data, by shifting the metrics by a single constant per fold. In \Cref{fig:rician-noise-pAUC-three} the unmodified partial Area Under the Free-Response Operating Characteristic curve (pAUC) values are shown in the \ieeeblue{left}\ panel, the pAUC values shifted per fold by the mean pAUC of the baseline ($\sigma = 0$) are shown in the \ieeeblue{middle}\ panel and the statistical significance p-values between the different Rician noise magnitudes are shown in the \ieeeblue{right}\ panel. Small amounts of Rician noise ($\sigma \in [0.01, 0.03]$) as data augmentation may improve lesion based model performance, but not with statistical significance ($P = 0.07-0.28$). 

\input{figures/rician-noise-pAUC-three}

% conclusion
The experiments suggest that Rician noise as data augmentation may improve both patient based and lesion based diagnostic performance, but neither metric improved with statistical significance. Based on prior experience from Kaggle challenges, I believe that intensity based data augmentations should be part of any data augmentation pipeline by default, and only taken out if motivated by experiments, rather than the other way around. This is also motivated by the data augmentation pipeline from the \namennUNet\ framework, which employs additive Gaussian noise, brightness, contrast and gamma augmentations as intensity based data augmentations for all datasets. While Rician noise at native resolution (before resampling the MRI sequences to a shared voxel spacing) is well suited for MRI in theory, the experiments in this appendix do not warrant rewriting a preprocessing pipeline to incorporate this specific augmentation. Instead of incorporating this single augmentation, it is probably more beneficial to adopt the data augmentation pipeline from \namennUNet, which has the standard geometric transformations, four intensity based augmentations, Gaussian blur and simulation of low resolution, all with magnitudes and probabilities backed by large-scale experiments. 
\subsection{Data}
%%%%%%%%%%%%%%%%%%
%% Introduction %%
%%%%%%%%%%%%%%%%%%
This appendix gives an overview of several data related projects during my internship. The aim of these projects was to improve the prostate MRI archive, annotations, metadata and study selection, and the goal of this appendix is to describe the changes made throughout the year and to provide documentation to future researchers. 

% intro section 1
The first section, \Cref{sec:preprocessing-RUMC-visits}, describes changes made to the preprocessing pipeline from DICOM archive to MHA scans. This section also highlights some of the design choices, to facilitate future improvements to the pipeline. 

% intro section 2
The second section, \Cref{sec:improving-RUMC-annotations}, describes improvements to the radiology based annotations of the RUMC dataset. This section also highlights efforts to improve the longevity of the annotation archive. 

% intro section 3
The third section, \Cref{sec:extracting-RUMC-metadata}, describes the extraction of Gleason scores from pathology reports, extraction of measurements from the radiology reports (prostate volume, PSA and PSA density) and extraction of prior Gleason scores and treatment from the radiology reports. 

% intro section 4
The fourth section, \Cref{sec:exclusion-criteria-RUMC}, describes the exclusion criteria employed for the RUMC dataset. This section also highlights the transparent pipeline for exclusion criteria. 

% intro section 5
The fifth and final section, \Cref{sec:preprocessing-UMCG-dataset}, describes the preparation of the UMCG dataset. Specifically, the naming scheme, study selection and naming errors are highlighted. 

%%%%%%%%%%%%%%%%%
%% RUMC images %%
%%%%%%%%%%%%%%%%%
\newcommand\seriesDescription{\texttt{series description}}
\newcommand\exampleSeriesDescriptionADC{\texttt{ep2d\_diff\_tra\_ADC\_DFC}}
\newcommand\exampleSeriesDescriptionTtwoW{\texttt{t2\_tse\_tra}}

\subsubsection{Preprocessing RUMC prostate MRI visits}
\label{sec:preprocessing-RUMC-visits}
The preprocessing pipeline from DICOM archive to MHA scans selects the relevant MRI sequences and combines the individual DICOM slices to a single MHA file per MRI sequence. The pipeline is configured to convert the axial T2-weighted (T2W), diffusion weighted (DWI), apparent diffusion coefficient (ADC), sagittal T2W and coronal T2W scans. 

% study selection
% Approach to select DICOM series:
% 1. Select the DICOM series which match the user-defined tags (per modality) and retain the series matching 
%   the DICOM series description with highest priority (first in list)
% 2. If multiple series matched, retain the series with the most slices (and at least min_num_slices slices). 
%   Note: this will NOT select a scan with isotropic voxel spacing (e.g., t2_spc_3D_cor_iso) over an anisotropic 
%   scan (e.g., t2_tse_cor), as the anisotropic tag has higher priority (in this example).
% 3. If multiple series matched, and have the same number of slices, select the DICOM series with the highest in-plane resolution.
% 4. If the above tie-breakers are insufficient, select the first one (possibly quasi-random due to side-effects)

MRI sequences in the DICOM archive are described by their \seriesDescription, which are tags that describe the sequence in a semi-structured manner. Common examples are \exampleSeriesDescriptionTtwoW\ for axial T2W and \exampleSeriesDescriptionADC\ for axial ADC scans, with 9214 and 8748 occurrences, respectively. In total, there are 1585 different \seriesDescription s, of which most have low frequency and/or refer to a T1-weighted sequence for dynamic contrast enhanced imaging. To determine which tags should be used, I visually inspected scans from various tags with high prevalence together with Matin. This resulted in the series descriptions shown in \Cref{tab:MRI-sequences}. 

In an ideal world, these \seriesDescription s would be sufficient to select the correct MRI sequence, but about 1/4th of the studies have multiple MRI sequences with the same \seriesDescription. This seemed to be mainly caused by download issues from the Picture Archiving and Communication System (PACS) to our storage system, where one series would be incomplete (missing DICOM slices) and the other complete. To account for the presence of both complete and incomplete series, I selected the series with most slices (within the same \seriesDescription). When multiple series have the same \seriesDescription\ and the same number of slices, I select the series with the highest in-plane resolution. 

The tags shown in \Cref{tab:MRI-sequences} and the sequence selection steps described above resulted in 9099 studies with axial T2W, ADC, DWI, sagittal T2W and coronal T2W scan between 2014 and 2020. 

Code for the improved preprocessing pipeline can be found \href{https://github.com/DIAGNijmegen/AbdomenMRUS-pca-surveillance/blob/dfd889da23d2cfb3a60e0fbe476f44399c1378ee/Environment/Dicom2MHD/dicom_archive.py}{\underline{here}} and \href{https://github.com/DIAGNijmegen/AbdomenMRUS-pca-surveillance/blob/dfd889da23d2cfb3a60e0fbe476f44399c1378ee/Preprocessing/Convert-DICOM-archive.ipynb}{\underline{here}}  (requires DIAG access). My contributions: 
\begin{itemize}
    \item Identified additional \seriesDescription s
    \item Sped up pipeline $16\times$, reducing total preprocessing time from approx. 8 days to approx. 12 hours
    \item Wrote documentation for preprocessing pipeline
    \item Solved bug where scans became scrambled or blank
    \item Solved bug where the \seriesDescription s where matched incorrectly (affected approx. 50 scans) 
    \item Wrote verification of MHA archive (mainly to ensure studies are properly written to disk)
    \item Delivered MHA archive with approx. 5000 new visits
\end{itemize}

\begin{table}[]
\caption{Series descriptions identified for T2W, ADC and high b-value}
\begin{tabular}{@{}lll@{}}
\toprule
\textbf{Sequence} & \textbf{Series description}                          & \textbf{Frequency} \\ \midrule
T2W axial         & t2\_tse\_tra                                         & 9214                 \\
                  & t2\_tse\_tra\_snel                                   & 5941                 \\
                  & t2\_tse\_tra\_snel\_bij bewogen t2 tra               & 1184                 \\ \midrule
ADC               & ep2d\_diff\_tra\_ADC\_DFC                            & 8748                 \\
                  & \begin{tabular}[c]{@{}l@{}}diff tra b 50 500 800 WIP511b alle \\ spoelen\_ADC\end{tabular}      & 256                  \\
                  & ep2d\_diff\_tra\_orig\_ADC\_DFC                      & 47                   \\
                  & ep2d\_diff\_tra\_ADC                                 & 46                   \\
                  & diff tra b 50 500 800 WIP511E\_ADC                   & 32                   \\ \midrule
High b-value      & ep2d\_diff\_tra\_CALC\_BVAL\_DFC                     & 8748                 \\
                  & \begin{tabular}[c]{@{}l@{}}diff tra b 50 500 800 WIP511b alle \\ spoelenCALC\_BVAL\end{tabular} & 256                  \\
                  & ep2d\_diff\_tra\_orig\_CALC\_BVAL\_DFC               & 47                   \\
                  & ep2d\_diff\_tra\_CALC\_BVAL                          & 46                   \\
                  & diff tra b 50 500 800 WIP511ECALC\_BVAL              & 32                   \\ \midrule
T2W coronal       & t2\_tse\_cor                                         & 8747                 \\
                  & t2\_spc\_3D\_cor\_iso                                & 463                  \\ \midrule
T2W sagittal      & t2\_tse\_sag                                         & 9214                 \\ \midrule
Do NOT use        & resolve\_diff\_tra\_CALC\_BVAL                       & 248                  \\
                  & resolve\_diff\_tra\_ADC                              & 248                  \\
                  & resolve\_diff\_b50\_400\_800\_tra\_CALC\_BVAL        & 37                   \\
                  & resolve\_diff\_b50\_400\_800\_tra\_ADC               & 37                   \\ \bottomrule
\end{tabular}
\label{tab:MRI-sequences}
\end{table}

%%%%%%%%%%%%%%%%%%%%%%
%% RUMC annotations %%
%%%%%%%%%%%%%%%%%%%%%%
\subsubsection{Improving RUMC annotations}
\label{sec:improving-RUMC-annotations}
Annotations are one of the most important ingredients for training deep neural networks. During my internship I've worked on improving the annotations though combining different sources of information. Most notably, I've automatically split the majority of the PI-RADS $\geq 4$ annotations in separate PI-RADS 4 or 5 labels, and identified \percentageIncorrectAnnotationsIdentified\ cases with incorrect annotation (\percentageIncorrectAnnotationsIdentified\ of all annotations). 

Splitting the annotations in separate labels for PI-RADS 4 or 5 allows to train a machine learning model with improved risk-stratification, by assigning a higher risk to PI-RADS 5 than to PI-RADS 4. Split annotations also allow more fine-grained meta-analysis, and paved the way to also annotate the PI-RADS 3 lesions as a separate label. The automatic conversion script was able to confidently split 3,540/3,652 ($97\%$) cases, leaving 112 cases. These 112 remaining cases have been manually split by Ilse, meaning the annotation archive is now completely split into PI-RADS 4 and 5. 

% comment:22: Splitting csPCa annotations into PI-RADS 4 or 5
% comment:29: Dataset conversion

My contributions: 
\begin{itemize}
    \item Automatically split 3,540/3,652 ($97\%$) PI-RADS $\geq 4$ annotations in either PI-RADS 4 or 5
    \item Orchestrated several (small) annotation projects with Ilse 
    \item Set up GitHub archive for annotations, which makes adding and revising annotations transparent
    \item Identified \numIncorrectAnnotationsIdentified\ incorrect annotations (\percentageIncorrectAnnotationsIdentified\ of total). 
\end{itemize}

%% Corrected delineations %%
% See the overview in Development/2021-07-27-overview-revised-annotations

%%%%%%%%%%%%%%%%%%%
%% RUMC metadata %%
%%%%%%%%%%%%%%%%%%%
\subsubsection{Extracting metadata from reports}
\label{sec:extracting-RUMC-metadata}
The dataset from RUMC is derived from clinical practice over the span of seven years, resulting in a lot of useful information, but not necessarily in a structured format. Reliable metadata for all studies is important for most downstream analyses, so during my internship I've set out to extract metadata from the radiology and pathology reports. The benefit of radiology and pathology reports is that those are available across all years, but the drawback is that reports are free form text. 

Apart from extracting PI-RADS scores from radiology reports, I've also extracted: 
\begin{itemize}
    \item Gleason scores and biopsy dates from pathology reports
    \item PSA level, PSA density, prostate volume, prior treatment and prior Gleason scores from radiology reports
\end{itemize}

The extraction method for this metadata is similar to the PI-RADS extraction described in \Cref{sec:automatic_finding_extraction}, albeit a bit simpler. Code can be found \href{https://github.com/DIAGNijmegen/AbdomenMRUS-pca-surveillance/blob/dfd889da23d2cfb3a60e0fbe476f44399c1378ee/Preprocessing/Enrich-Metadata.ipynb}{\underline{here}} (requires DIAG access). 

\input{figures/STARD-RUMC}
% comment:15
% comment:23
% comment:36: Automatic extraction of PI-RADS scores from radiology reports

%%%%%%%%%%%%%%%%%%%%%%%%%%%%%
%% RUMC exclusion criteria %%
%%%%%%%%%%%%%%%%%%%%%%%%%%%%%
\subsubsection{Exclusion criteria RUMC}
\label{sec:exclusion-criteria-RUMC}
Studies with treatment or a positive biopsy (Gleason score $\geq 3+4$) prior to the MRI scan are excluded, as well as studies with bad MRI scan quality and studies from patients who opted out. 
To identify studies with prior treatment, I started with the list of treatments used by Matin, and extended that list by looking for additional treatments in the radiology reports. 
The list of treatments can be found in \Cref{tab:excluded-treatments}. 
I also excluded follow-up studies, even if the subsequent report didn't repeat the prior treatment. 
The improved pipelin resulted in identifying an additional \additionalTreatmentsFound\ studies with prior treatment (\additionalTreatmentsFoundPercentage\ more). 

Further documentation, details and lists of excluded studies can be found \href{https://github.com/DIAGNijmegen/AbdomenMRUS-pca-surveillance/blob/dfd889da23d2cfb3a60e0fbe476f44399c1378ee/Environment/config/exclusion_criteria.py}{\underline{here}} (requires DIAG access). The STARD diagram showing the number of studies included and excluded in this work is shown in \Cref{fig:STARD-RUMC}. 
% comment:19
% comment:20
% comment:24: Exclusion criteria: prior treatment and image artifacts

\begin{table}[]
\caption{Excluded treatments}
\begin{tabular}{@{}lll@{}}
\toprule
\textbf{Previously matched treatments}      & \textbf{Additional treatments} &  \\ \midrule
RALP                                        & TUR                            &  \\
Robotic-assisted laparoscopic prostatectomy & laser focale                   &  \\
laparoscopic                                & TULSA                          &  \\
radiotherapie                               & prostectomie                   &  \\
radiation                                   & focale behandeling             &  \\
radiotherapy                                & MRI laser behandeling          &  \\
HIFU                                        & bestraling                     &  \\
prostectomy                                 & hemi-ablatie                   &  \\
TURP                                        & ablatie                        &  \\
resection                                   & laserablatie                   &  \\
cryo                                        & anteriorresectie               &  \\
prostatectomie                              & sigmoidresectie                &  \\
brachytherapie                              & Green light laser              &  \\
therapie                                    & TURT                           &  \\
resectie                                    & chemotherapie                  &  \\
RRP                                         & LHRH                           &  \\
radicale prostatectomy                      &                                &  \\
prostatectomy                               &                                &  \\
EBRT                                        &                                &  \\
radiation therapy                           &                                &  \\
chemoradiatie                               &                                &  \\
na de chirurgie                             &                                &  \\
chirurgie                                   &                                &  \\
Hormonen                                    &                                &  \\
TURS                                        &                                &  \\ \bottomrule
\end{tabular}
\label{tab:excluded-treatments}
\end{table}

%%%%%%%%%%
%% UMCG %%
%%%%%%%%%%
\subsubsection{UMCG dataset}
\label{sec:preprocessing-UMCG-dataset}
The dataset from UMCG remained unused in my project, but I did prepare it. This involved collaborating with Jeroen and Christian to receive additional metadata, documentation and understanding their naming scheme. Furthermore, I extended the preprocessing pipeline described in \Cref{sec:preprocessing-RUMC-visits} to harmonise the datasets from UMCG and RUMC. The prepared dataset and documentation can be found at \verb!Chansey::pelvis/data/prostate-MRI/umcg/!. Code can be found \href{https://github.com/DIAGNijmegen/AbdomenMRUS-pca-surveillance/blob/dfd889da23d2cfb3a60e0fbe476f44399c1378ee/Preprocessing/Convert-RUMC-Annotations.ipynb}{\underline{here}} and \href{https://github.com/DIAGNijmegen/AbdomenMRUS-pca-surveillance/blob/dfd889da23d2cfb3a60e0fbe476f44399c1378ee/Preprocessing/Convert-UMCG-archive.ipynb}{\underline{here}} (requires DIAG access). 

Visits in our internal RUMC dataset are identified by a unique patient identifier and a unique study identifier. Using these two identifiers, it is straightforward to identify which studies belong to the same patient, and new visits can be added to the archive without affecting the naming scheme of existing visits. A similar naming scheme can be constructed for the UMCG dataset using their markdatasheet. 

\newcommand\patientID{\texttt{anon\_id}}
\newcommand\visitNum{\texttt{ret\_pat\_number}}
\newcommand\redcapID{\texttt{redcap\_id}}
\newcommand\studyID{\texttt{[redcap\_id]-[ret\_pat\_number]}}
Visits in the external UMCG dataset can be uniquely identified using the \redcapID\ (1 to 965) and \visitNum\ (empty for first visit, 1 for second visit and 2 for third visit), and patients can be uniquely identified using the \patientID\ (e.g., M-001 or U-001). To harmonise the naming scheme with the RUMC dataset, the \redcapID\ and \visitNum\ are combined to a unique study identifier as \studyID, where an empty \visitNum\ is replaced by a zero.

% patient id: M-ddd or U-ddd, with ddd a three-digit number. 
% visit num: empty for first visit, 1 for second, 2 for third, ...
% redcap id: identifier for (a sequence of) visits of a patients

The UMCG dataset consists of MRI examinations from UMCG, Martini Ziekenhuis and peripheral hospitals throughout the province of Groningen. Studies from UMCG or Martini have \texttt{mri\_location\_1 == 1}, while studies from peripheral hospitals have \texttt{mri\_location\_1 == 2}, with the specific peripheral hospital described in \texttt{mri\_location\_2}. Studies from peripheral hospitals have large variance in acquisition parameters, so only including studies from UMCG or Martini may be recommended. 

Further study selection criteria are prior treatment, prior positive biopsies and bad scan quality. 
Prior treatment was an exclusion criteria for the UMCG dataset, so none of the studies we received should have prior treatment. Bad scan quality wasn't an explicit exclusion criterion, but scans that are of insufficient quality for interpretation are usually repeated, and if all went well we only received good scans. To exclude studies with previously confirmed prostate cancer we received an updated markdatasheet, with prior Gleason scores described in \texttt{prev\_tar\_gleas1}, \texttt{prev\_tar\_gleas2}, \texttt{prev\_trus\_g1} and \texttt{prev\_trus\_g2}. 

Although the UMCG dataset is of very high quality, it did contain several naming inconsistencies in its files, likely caused by manual typing errors. To resolve these inconsistencies in a transparent manner, Anindo and I created a \href{https://github.com/DIAGNijmegen/prostateMR_archive_umcg}{\underline{repository}} for the annotations and corrected the typing mistakes. 

\subsection{Active Surveillance}
Active Surveillance within prostate cancer management is an interesting and important direction to improve patient care. Working on deep learning solutions for Active Surveillance patients has taught me a lot, but did not result in concrete results. This lack of results was mainly caused by insufficient clinical motivation for the desired outcome. While existing Active Surveillance programs have shown excellent low prostate cancer mortality \citep{welty2015extended, selvadurai2013medium, klotz2015long, tosoian2015intermediate, bokhorst2016decade}, it is still relatively new. As a result, there is no clear target objective that a deep learning solution should aim for. 

Several options for target objectives exist: 
\begin{enumerate}
    \item Progression from Gleason grade group $\leq 1$ to Gleason grade group $\geq 2$
    \item Progression of PI-RADS score
    \item Identify new or vanished lesions
    \item Change of mean/min/std. ADC values within lesion mask
    \item Progression of lesion volume
\end{enumerate}

Unfortunately, all targets have limitations. Only few patients undergo multiple biopsies (1); PI-RADS scores suffer from large inter- and intra-reader variability, which is amplify when deriving change (2 \& 3); contours of lesions are often ill-defined, resulting in unstable statistics and volume (4 \& 5). 

The interested reader is encouraged to contact me (\href{mailto:Joeran.Bosma@radboudumc.nl}{Joeran.Bosma@radboudumc.nl}) for further discussions about Active Surveillance within prostate cancer management, and/or read the literature review I wrote on the deep learning side of it (\href{https://bosma.co/Bosma2021deep.pdf}{bosma.co/Bosma2021deep.pdf}. 

% Literature review: bosma.co/Bosma2021deep.pdf

\subsection{Image registration}
Image registration is a technique that can align medical scans that are similar but not exactly the same, which can be extremely helpful for a baseline and follow-up scan. 
An example is shown in \Cref{fig:registration-example}, where the first and third panel show the baseline and follow-up visits, and the second panel shows the baseline scan aligned to the follow-up scan. To align the baseline scan, it is moved `up' (towards anterior) and `pulled out of the page' (towards base), resulting in an aligned prostate. 

During my investigation of image registration for prostate MRI, I learned three practical lessons which I'd like to share:
\begin{enumerate}
    \item Normalise your scans before registration. Similar to deep learning, an image registration algorithm uses gradient ascent to optimise a similarity metric, and a registration can completely fail if those gradients are e.g. 1000 times higher than expected. 
    \item Registering the prostate segmentation masks, rather than the original scans, gives the most robust registration. A fine-grained registration of the original scans can then be compared to the robust registration, to spot cases where the fine-grained registration completely failed. 
    \item The structural similarity index metric (SSIM) is the metric that corresponds best with the true displacement, as shown by my brother \citep{bosma2021quantitative}. 
\end{enumerate}

% Image registration is difficult to quantitatively evaluate, 
% When I was working on Active Surveillance within prostate cancer diagnosis, I investigated image registration

\input{figures/registration-example}
\subsection{Dynamic candidate extraction from softmax predictions}
When I started my internship, the method to extract lesion candidates from a model's softmax prediction involved a static threshold. Below this threshold, all model predictions were set to zero, and the remaining `islands' would then be the lesion candidates. This threshold was static across all samples, even though different models and even different datasets have different optimal thresholds. Other than tuning the static threshold for each model and dataset, there was no way to deduce a proper threshold. 

To circumvent the limitation of a static candidate extraction, I proposed a sample-dependent `dynamic' candidate extraction. This candidate extraction pipeline should extract `blobs' from the softmax prediction in a scale-free manner. The method I proposed defines a lesion candidate by selecting the most confident voxel as the `peak' and extending the lesion candidate until $40\%$ of its peak confidence. To extract multiple lesion candidates, this process is repeated. See \Cref{fig:dynamic-threshold-pipeline-large} for an example. 

\input{figures/dynamic-threshold-pipeline-large}

To validate the dynamic extraction of lesion candidates, I compared model performance obtained using the dynamic extraction pipeline against a range of static thresholds, as well as a sample-dependent threshold obtained using Otsu's method and a sample-dependent threshold defined as $40\%$ of the sample's peak. Please note that the latter method is different from the dynamic pipeline because it applies a single threshold and extracts all subsequent `islands', instead of the iterative approach of the dynamic extraction, and is termed `dynamic-fast'. Results for my baseline models (at the time of investigating the dynamic lesion candidate extraction), with 5-fold cross-validation and 5 restarts are shown in \Cref{fig:dynamic-threshold-FROC-performance}. Results for my models trained on automatic annotations (which used soft labels at the time), with 5-fold cross-validation and 3 restarts are shown in \Cref{fig:dynamic-threshold-FROC-performance-AVA}. The dynamic lesion candidate extraction either performs on par or outperforms the best static threshold, across all metrics. Most importantly, the dynamic extraction did not require any tuning, while the static pipeline has different optimal thresholds across metrics and models.

\input{figures/dynamic-threshold-FROC-performance}
\input{figures/dynamic-threshold-FROC-performance-pseudo-labels}
