# Supplementary material for: Annotation-efficient cancer detection with report-guided lesion annotation for deep learning-based prostate cancer detection in bpMRI
Source: arXiv:2112.05151 source file (2022-02-19)
Supplement: Supplementary file 4 [file 2a-parse-report.tex]

\section{Extraction of Report Findings}
First, we tried to split the radiology reports in sections for individual findings, by searching for text that matches the following structure:
% make verbatim spacing less and change back to 'optional number indicator'?
\begin{verbatim}
[Finding] (number indicator) [number]
\end{verbatim}
Where `Finding' matches the Dutch translations \textit{`afwijking'}, \textit{`laesie'}, \textit{`markering'} or \textit{`regio'}. 
% Where \verb!Finding! matches the Dutch translations \verb!Afwijking!, \verb!Laesie!, \verb!Markering! or \verb!Regio!. 
The optional number indicators are \textit{`nr.'}, \textit{`mark'} and \textit{`nummer'}. The number at the end matches one or multiple numbers (e.g., \textit{`1'} or \textit{`2+3'}).

% For reference, the pattern to split reports in sections is:
% (Afwijking|Index laesie|Markering|Regio|Laesie) *(nr\.?)? *(mark)? *((in)? nummer)? *(\d+)\+?(\d+)?\+?(\d+)?\+?(\d+)?

% Secondly, if the report was split in sections successfully, we extract the PI-RADS scores. To extract the PI-RADS score we search for text that matches: 
Secondly, we extracted the PI-RADS scores by searching for text that matches the following structure: 
% make verbatim spacing less and change back to 'optional separators'?
\begin{verbatim}
[PI-RADS] (separators) [number 1-5]
\end{verbatim}
Where the optional separators include \textit{`v2 category'} and `\verb!:!'. The dash between \textit{`PI'} and \textit{`RADS'} is optional. The T2W, DWI and DCE scores, which define the PI-RADS score, are extracted analogous to the PI-RADS score, while also allowing joint extraction: %. When the scores are reported jointly, they are automatically matched to the respective with an important addition. The T2W, DWI and DCE scores are often reported jointly like:
\begin{verbatim}
T2W/DWI/DCE score: [1-5]/[1-5]/[-+]
\end{verbatim}
In this instance, the first number is matched with the T2W score, the second with DWI and the \verb!+! or \verb!-! with DCE. 

In case the report could not be split in sections per lesion, we applied strict pattern matching on the full report. During strict pattern matching we only extract T2W, DWI and DCE scores jointly, to ensure the scores are from the same lesion. The resulting PI-RADS scores were extracted from the full report and matched to the individual scores.
