# Supplementary material for: Annotation-efficient cancer detection with report-guided lesion annotation for deep learning-based prostate cancer detection in bpMRI
Source: arXiv:2112.05151 source file (2022-02-19)
Supplement: Supplementary file 5 [file 2b-detection-architecture.tex]

\section{Detection Model Architecture}
\label{sec:detection_model_architectures}
For our prostate cancer segmentation task, \namennUNet\ [1] configured itself to use a 3D \nameUNet\ with five down-sampling steps, as shown in \Cref{fig:detector_networks}. This figure also shows the specific choice of 2D/3D convolutional blocks, max-pooling layers and transposed convolutions. % is best conveyed based on the figure.  
No cascade of \nameUNets\ or 2D \nameUNet\ was triggered for our dataset. 

% Specifically, the anisotropic \nameUNet\ has two down-sampling steps where the pooling and convolutions happen in 2D, followed by two down-sampling steps where both pooling and convolutions happen in 3D, and finally one down-sampling step with pooling in 2D and convolutions in 3D. Each convolutional block contains two convolutional layers with kernel size $1\times 3\times 3$ in 2D and kernel size $3\times 3\times 3$ in 3D. 
% No cascade of \nameUNets\ or 2D \nameUNet\ was triggered for our dataset. 

The implementation of the \nameUNetagpp\ architecture is the same as in [2], with the exception of \nameLeakyReLU\ [3] activation \added{functions}\ throughout the decoder and decreased $L_2$ kernel regularisation of $10^{-4}$. See [2] for implementation details. 

~
~
\makeatletter
\newcommand*{\wackyenum}[1]{%
  \expandafter\@wackyenum\csname c@#1\endcsname%
}

\newcommand*{\@wackyenum}[1]{%
  $\ifcase#1\or[1]\or[2]\or[3]\or42%
    \else\@ctrerr\fi$%
}
\AddEnumerateCounter{\wackyenum}{\@wackyenum}{53.13}
\makeatother

\begin{enumerate}[label=\wackyenum*]
\item F. Isensee, P. F. Jaeger, S. A. Kohl, J. Petersen, and K. H. Maier-Hein, ``nnU-Net: a self-configuring method for deep learning-based biomedical image segmentation,'' Nature Methods, vol. 18, no. 2, pp. 203--211, 2021. 
\item A. Saha, M. Hosseinzadeh, and H. Huisman, ``{End-to-end Prostate Cancer Detection in bpMRI via 3D CNNs: Effects of Attention Mechanisms, Clinical Priori and Decoupled False Positive Reduction}'', \textit{Medical Image Analysis}, p. 102 155, 2021, ISSN: 1361-8415.
\item A. L. Maas, A. Y. Hannun, and A. Y. Ng, ``Rectifier Nonlinearities Improve Neural Network Acoustic Models'', in \textit{Proc. icml, Citeseer}, vol. 30, 2013, p. 3.
\end{enumerate}
