# Supplementary material for: Annotation-efficient cancer detection with report-guided lesion annotation for deep learning-based prostate cancer detection in bpMRI
Source: arXiv:2112.05151 source file (2022-02-19)
Supplement: Supplementary file 6 [file a-STARD.tex]

\subsection{STARD diagram}
\blue{PENDING}.
