# Supplementary material for: Annotation-efficient cancer detection with report-guided lesion annotation for deep learning-based prostate cancer detection in bpMRI
Source: arXiv:2112.05151 source file (2022-02-19)
Supplement: Supplementary file 7 [file b-detection-model.tex]

\subsection{Detection Model Architecture}
\label{sec:detection_model_architectures}
For our prostate cancer segmentation task, \namennUNet\ configured itself to use a 3D \nameUNet\ with five down-sampling steps, as shown in \Cref{fig:detector_networks}. This figure also shows the specific choice of 2D/3D convolutional blocks, max-pooling layers and transposed convolutions. % is best conveyed based on the figure.  
No cascade of \nameUNets\ or 2D \nameUNet\ was triggered for our dataset. 

% Specifically, the anisotropic \nameUNet\ has two down-sampling steps where the pooling and convolutions happen in 2D, followed by two down-sampling steps where both pooling and convolutions happen in 3D, and finally one down-sampling step with pooling in 2D and convolutions in 3D. Each convolutional block contains two convolutional layers with kernel size $1\times 3\times 3$ in 2D and kernel size $3\times 3\times 3$ in 3D. 
% No cascade of \nameUNets\ or 2D \nameUNet\ was triggered for our dataset. 

The implementation of the \nameUNetagpp\ architecture is the same as in \citep{saha2021end}, with the exception of \nameLeakyReLU\ \citep{maas2013rectifier} activations throughout the decoder and decreased $L_2$ kernel regularisation of $10^{-4}$. See \citep{saha2021end} for implementation details. 

\begin{figure*}[t!]
    \centering
    \includegraphics[width=\textwidth]{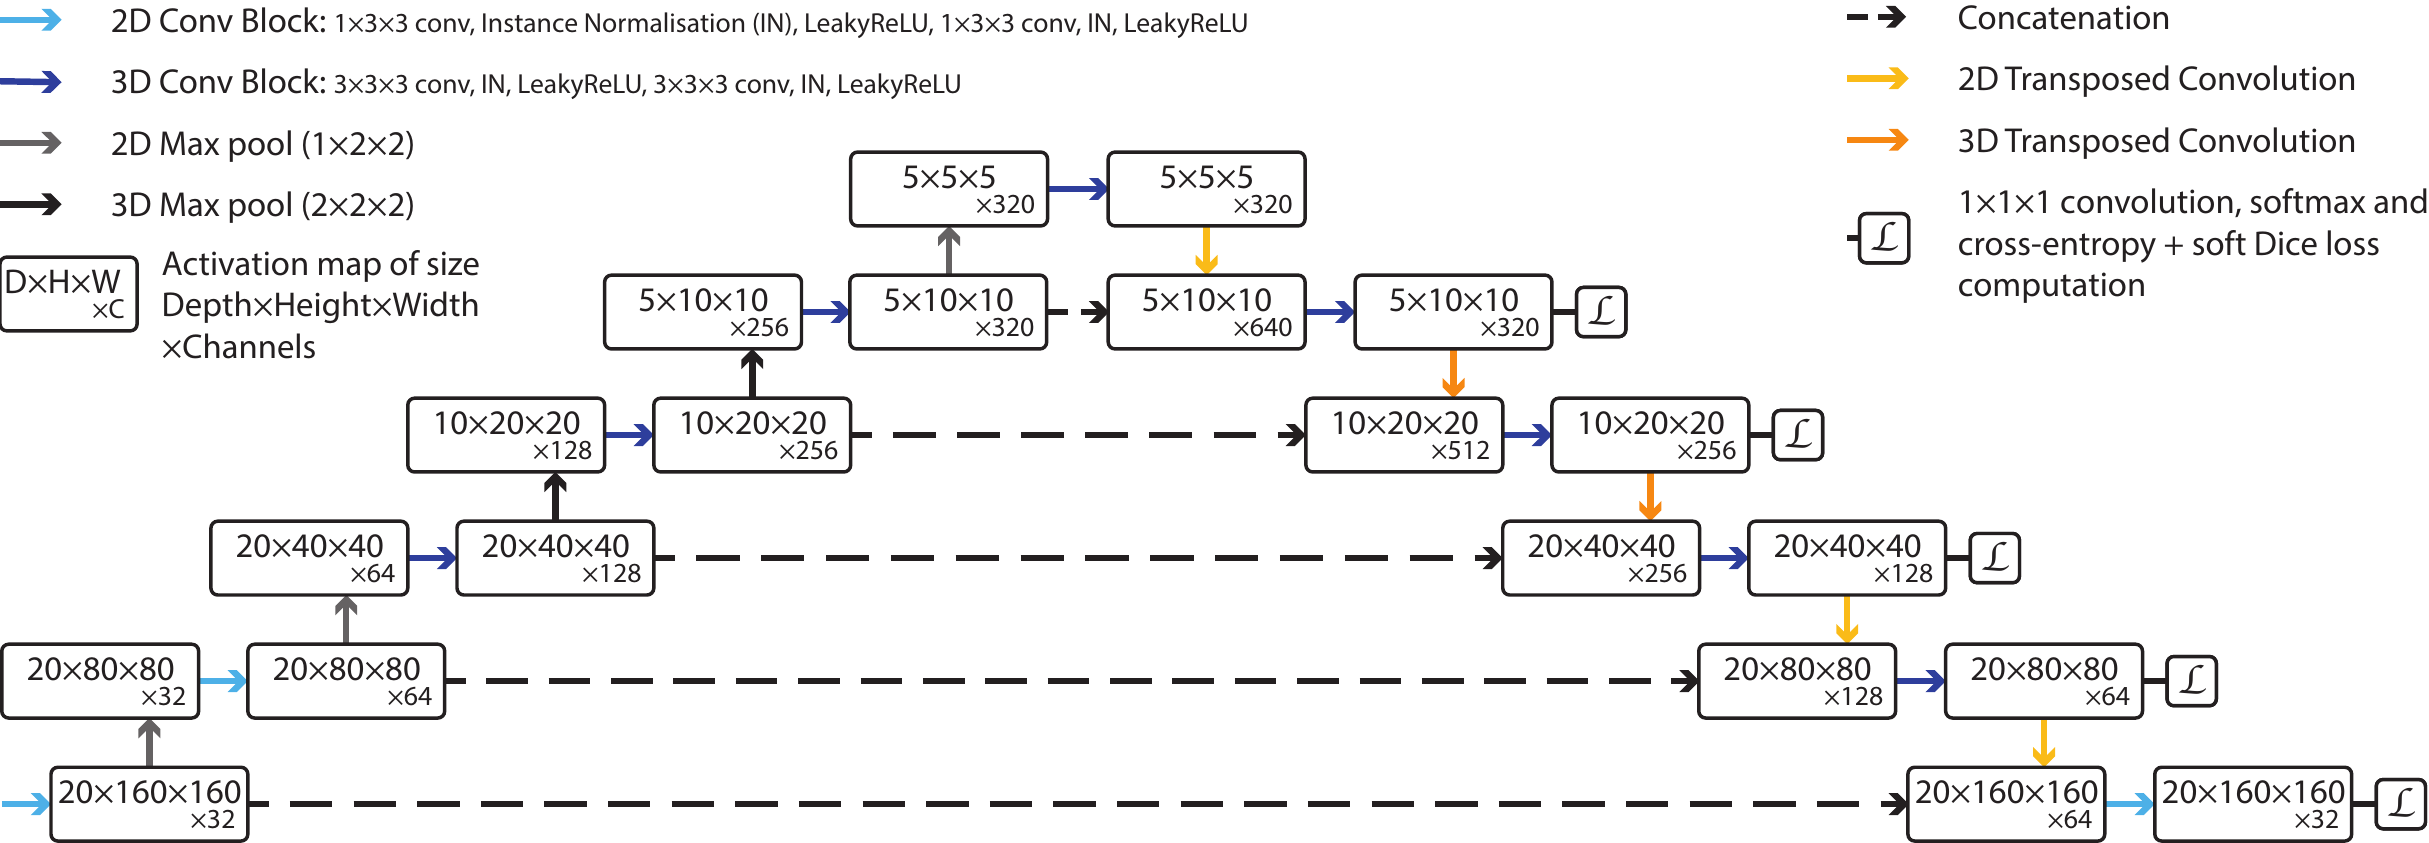}
    \caption{Architecture schematic of the \namennUNet, as configured for our prostate cancer segmentation task. }
    \label{fig:detector_networks}
\end{figure*}
