# Supplementary material for: Annotation-efficient cancer detection with report-guided lesion annotation for deep learning-based prostate cancer detection in bpMRI
Source: arXiv:2112.05151 source file (2022-02-19)
Supplement: Supplementary file 8 [file c-augmentation-overview.tex]

\subsection{Augmentations}
\begin{table*}[!t]
\caption{\label{tab1}Data augmentations used during model training}
\centering
\begin{tabular}{l|ll|ll}
\toprule
Model                                               & \multicolumn{2}{c|}{\nameUNetagpp}  & \multicolumn{2}{c}{\namennUNet}                                                                                     \\ \hline
Normalisation                                              & \multicolumn{2}{l|}{(Instance-wise) min/max}           & \multicolumn{2}{l}{(Instance-wise) zero mean, unit variance}                                                                                                     \\ \hline
Augmentation                                               &  Distribution                                  & Probability       & Distribution                                         & Probability       \\ \hline
Mirror                                                     & Horizontal           & $50\%$ shared     & All axes                                                                                            & $50\%$ individual \\
Rotation (degrees)                                         & $7.5\cdot\mathcal{N}(0, 1)$   & $50\%$ shared     & $\mathcal{U}(-180, 180)$                                                                       & $20\%$ individual \\
Zoom (affine scaling factor)                               & $1.05\cdot\mathcal{N}(0, 1)$  & $50\%$ shared     & $\mathcal{U}(0.7, 1.4)$                                                                        & $20\%$ individual \\
Translation, horizontal                                    & $0.05 \cdot\mathcal{N}(0, 1)$ & $50\%$ shared     & -                                                                                                   & -                 \\
Translation, vertical                                      & $0.05 \cdot\mathcal{N}(0, 1)$ & $50\%$ shared     & -                                                                                                   & -                 \\
Additive noise                                       & $\text{Rician}(\sigma=0.01)$         & $75\%$ individual & $\mathcal{N}(0, \sigma)$, with $\sigma \sim \mathcal{U}(0, 0.1)$                               & $15\%$ individual \\
Gaussian blur                                              & -                                  & -                 & See \citep{isensee2021nnu}, Sup. Mat. Note 4                                 & $20\%$ individual \\
Brightness                                           & -                                  & -                 & $\mathcal{U}(0.7, 1.3)$                                                                        & $15\%$ individual \\
Contrast                                                   & -                                  & -                 & $\mathcal{U}(0.65, 1.5)$, with subsequent clipping & $15\%$ individual \\
Simulation of low resolution                               & -                                  & -                 & See \citep{isensee2021nnu}, Sup. Mat. Note 4                                 & $25\%$ individual \\
Gamma augmentation                                         & -                                  & -                 & See \citep{isensee2021nnu}, Sup. Mat. Note 4                                 & $15\%$ individual
\end{tabular}
\end{table*}
