# Supplementary material for: Annotation-efficient cancer detection with report-guided lesion annotation for deep learning-based prostate cancer detection in bpMRI
Source: arXiv:2112.05151 source file (2022-02-19)
Supplement: Supplementary file 10 [file a-rician-noise.tex]

\subsection{Rician noise}
% introduce data augmentations
Data augmentation is one of the most import techniques to improve the generalisation of deep learning models to unseen data. Typical data augmentations include rotation, mirroring, translation and zooming, but many more exist. When training a network with data augmentations, the training samples are transformed with one or multiple augmentations before being provided to the network. As a result, the network is guided to make its predictions invariant under these transformations, which results in a model that generalises better to unseen data. 

% introduce intensity based augmentations
At the start of my internship, the group's data augmentation pipeline consisted of rotation, translation, horizontal flipping and zooming, which are all geometric transformations. To improve the data augmentation pipeline, I have investigated intensity based augmentations, which are complementary to geometric transformations. While geometric transformations move the original voxels around in some structured way, intensity based augmentations preserve the location of the voxels and apply noise to each voxel. 

% introduce Rician noise
Intensity based augmentations span a large domain of additive, multiplicative and/or any nonlinear function based on the original voxel value. %  and/or multiplicative noise, with noise parameters drawn from any distribution. 
One of the best known intensity based augmentations is additive Gaussian noise, where noise following the Gaussian distribution is added to each voxel individually:
\begin{equation}
    I_{new} = I_{old} + \mathcal{N}(0, \sigma^2)
\end{equation}
Where $\mathcal{N}$ is the Gaussian distribution and $\sigma^2$ the variance. 

A drawback of additive Gaussian noise is that the intensities can become negative, which is physically impossible for MRI sequences such as T2W and DWI (these scans as used by radiologists and this work are magnitude maps; phase maps can be negative, but are typically disregarded). Noise in MRI scans is shown to be governed by the Rician distribution \citep{gudbjartsson1995rician}, which is non-negative and approaches the Gaussian distribution for large values. The Rician distribution is given by:
\begin{equation}
    I_{new} = \sqrt{(I_{old} + \sigma \cdot \phi)^2 + (\sigma\cdot\phi)2}
\end{equation}
Where $\sigma$ is the magnitude of the Rician distribution and $\phi$ is drawn from $\mathcal{N}(0, 1)$ for each voxel individually.

\newcommand\footnoteMisalignment{\footnote{Accounting for the misalignment proved difficult, so I excluded \numVisitsMisalignedExcluded\ cases ($1.6\%$) which otherwise would have a misalignment of at least 2 mm. }}

% introduce dynamic preprocessing pipeline
Motivated by the physical relevance of the Rician distribution, I have adapted the data pipeline to incorporate this distribution as data augmentation. This required an overhaul of the way the scans are preprocessed, because the Rician noise needs to be applied at native resolution and initially the scans were resampled at an early stage. The new preprocessing pipeline saves the scans at original resolution, and resamples them on-the-fly during model training, after applying the Rician noise data augmentation. This overhaul also resulted in a good understanding of the preprocessing steps, which led to the discovery of a bug where T2W and ADC/DWI scans became misaligned due to the preprocessing pipeline\footnoteMisalignment.

% introduce experiment
To determine a good magnitude for the Rician noise ($\sigma$), I identified the range of $\sigma \in [0, 0.05]$ as relevant values through visual inspection, and tested $\sigma=0.00$, $0.01$, $0.02$, $0.03$, $0.04$ and $0.05$. During training, the Rician noise is applied with a probability of $75\%$. For each magnitude, models were trained with 5-fold cross-validation and 2 restarts. The resulting 10 performance metrics were compared using the permutation test with \numIterationsPermutationTest\ iterations. To retain the integrity of the external test set (ZGT), each model is evaluated on the RUMC dataset. 

% results
To evaluate the patient based diagnostic performance we can leverage the \numUnlabelledStudiesFullDataset\ unlabelled RUMC visits, which results in a much more stable evaluation compared to the $\approx 300$ labelled studies in each validation fold\footnote{This number is lower than 1/5th of all labelled samples, because samples with positive MRI (PI-RADS $\geq 3$) but unknown biopsy result were excluded from the validation set. }. For these unlabelled visits the ground truth is derived by automatically extracting the scores from pathology and radiology reports. To construct labels with low error rate and typical distribution of low-, intermediate and high risk patients, a method similar to ProstateX was employed: cases with Gleason grade group $\geq 2$ are positive and cases with either Gleason grade group $\leq 1$ or PI-RADS $\leq 2$ are negative. This gives 883 biopsy-confirmed positive cases and 2,656 negative cases. 

The patient based diagnostic performances as evaluated against the ProstateX-like labels are given in \Cref{fig:rician-noise-AUC-performance}. The statistical significance p-values are given in \Cref{fig:rician-noise-AUC-significance-matrix}. Small amounts of Rician noise ($\sigma \in [0.01, 0.03]$) as data augmentation may improve patient based model performance, but not with statistical significance ($P = 0.17-0.55$). 
\input{figures/rician-noise-AUC-performance}
\input{figures/rician-noise-AUC-significance-matrix}

To evaluate lesion based diagnostic performance, manually annotated cases are required. The 5-fold cross-validation results in five validation sets with small differences in difficulty, resulting is slightly higher or lower performance metrics across all models for some validation folds. Differences in model performance can be highlighted by accounting for this variation intrinsic to the data, by shifting the metrics by a single constant per fold. In \Cref{fig:rician-noise-pAUC-three} the unmodified partial Area Under the Free-Response Operating Characteristic curve (pAUC) values are shown in the \ieeeblue{left}\ panel, the pAUC values shifted per fold by the mean pAUC of the baseline ($\sigma = 0$) are shown in the \ieeeblue{middle}\ panel and the statistical significance p-values between the different Rician noise magnitudes are shown in the \ieeeblue{right}\ panel. Small amounts of Rician noise ($\sigma \in [0.01, 0.03]$) as data augmentation may improve lesion based model performance, but not with statistical significance ($P = 0.07-0.28$). 

\input{figures/rician-noise-pAUC-three}

% conclusion
The experiments suggest that Rician noise as data augmentation may improve both patient based and lesion based diagnostic performance, but neither metric improved with statistical significance. Based on prior experience from Kaggle challenges, I believe that intensity based data augmentations should be part of any data augmentation pipeline by default, and only taken out if motivated by experiments, rather than the other way around. This is also motivated by the data augmentation pipeline from the \namennUNet\ framework, which employs additive Gaussian noise, brightness, contrast and gamma augmentations as intensity based data augmentations for all datasets. While Rician noise at native resolution (before resampling the MRI sequences to a shared voxel spacing) is well suited for MRI in theory, the experiments in this appendix do not warrant rewriting a preprocessing pipeline to incorporate this specific augmentation. Instead of incorporating this single augmentation, it is probably more beneficial to adopt the data augmentation pipeline from \namennUNet, which has the standard geometric transformations, four intensity based augmentations, Gaussian blur and simulation of low resolution, all with magnitudes and probabilities backed by large-scale experiments.
