# Supplementary material for: Annotation-efficient cancer detection with report-guided lesion annotation for deep learning-based prostate cancer detection in bpMRI
Source: arXiv:2112.05151 source file (2022-02-19)
Supplement: Supplementary file 11 [file b-data.tex]

\subsection{Data}
%%%%%%%%%%%%%%%%%%
%% Introduction %%
%%%%%%%%%%%%%%%%%%
This appendix gives an overview of several data related projects during my internship. The aim of these projects was to improve the prostate MRI archive, annotations, metadata and study selection, and the goal of this appendix is to describe the changes made throughout the year and to provide documentation to future researchers. 

% intro section 1
The first section, \Cref{sec:preprocessing-RUMC-visits}, describes changes made to the preprocessing pipeline from DICOM archive to MHA scans. This section also highlights some of the design choices, to facilitate future improvements to the pipeline. 

% intro section 2
The second section, \Cref{sec:improving-RUMC-annotations}, describes improvements to the radiology based annotations of the RUMC dataset. This section also highlights efforts to improve the longevity of the annotation archive. 

% intro section 3
The third section, \Cref{sec:extracting-RUMC-metadata}, describes the extraction of Gleason scores from pathology reports, extraction of measurements from the radiology reports (prostate volume, PSA and PSA density) and extraction of prior Gleason scores and treatment from the radiology reports. 

% intro section 4
The fourth section, \Cref{sec:exclusion-criteria-RUMC}, describes the exclusion criteria employed for the RUMC dataset. This section also highlights the transparent pipeline for exclusion criteria. 

% intro section 5
The fifth and final section, \Cref{sec:preprocessing-UMCG-dataset}, describes the preparation of the UMCG dataset. Specifically, the naming scheme, study selection and naming errors are highlighted. 

%%%%%%%%%%%%%%%%%
%% RUMC images %%
%%%%%%%%%%%%%%%%%
\newcommand\seriesDescription{\texttt{series description}}
\newcommand\exampleSeriesDescriptionADC{\texttt{ep2d\_diff\_tra\_ADC\_DFC}}
\newcommand\exampleSeriesDescriptionTtwoW{\texttt{t2\_tse\_tra}}

\subsubsection{Preprocessing RUMC prostate MRI visits}
\label{sec:preprocessing-RUMC-visits}
The preprocessing pipeline from DICOM archive to MHA scans selects the relevant MRI sequences and combines the individual DICOM slices to a single MHA file per MRI sequence. The pipeline is configured to convert the axial T2-weighted (T2W), diffusion weighted (DWI), apparent diffusion coefficient (ADC), sagittal T2W and coronal T2W scans. 

% study selection
% Approach to select DICOM series:
% 1. Select the DICOM series which match the user-defined tags (per modality) and retain the series matching 
%   the DICOM series description with highest priority (first in list)
% 2. If multiple series matched, retain the series with the most slices (and at least min_num_slices slices). 
%   Note: this will NOT select a scan with isotropic voxel spacing (e.g., t2_spc_3D_cor_iso) over an anisotropic 
%   scan (e.g., t2_tse_cor), as the anisotropic tag has higher priority (in this example).
% 3. If multiple series matched, and have the same number of slices, select the DICOM series with the highest in-plane resolution.
% 4. If the above tie-breakers are insufficient, select the first one (possibly quasi-random due to side-effects)

MRI sequences in the DICOM archive are described by their \seriesDescription, which are tags that describe the sequence in a semi-structured manner. Common examples are \exampleSeriesDescriptionTtwoW\ for axial T2W and \exampleSeriesDescriptionADC\ for axial ADC scans, with 9214 and 8748 occurrences, respectively. In total, there are 1585 different \seriesDescription s, of which most have low frequency and/or refer to a T1-weighted sequence for dynamic contrast enhanced imaging. To determine which tags should be used, I visually inspected scans from various tags with high prevalence together with Matin. This resulted in the series descriptions shown in \Cref{tab:MRI-sequences}. 

In an ideal world, these \seriesDescription s would be sufficient to select the correct MRI sequence, but about 1/4th of the studies have multiple MRI sequences with the same \seriesDescription. This seemed to be mainly caused by download issues from the Picture Archiving and Communication System (PACS) to our storage system, where one series would be incomplete (missing DICOM slices) and the other complete. To account for the presence of both complete and incomplete series, I selected the series with most slices (within the same \seriesDescription). When multiple series have the same \seriesDescription\ and the same number of slices, I select the series with the highest in-plane resolution. 

The tags shown in \Cref{tab:MRI-sequences} and the sequence selection steps described above resulted in 9099 studies with axial T2W, ADC, DWI, sagittal T2W and coronal T2W scan between 2014 and 2020. 

Code for the improved preprocessing pipeline can be found \href{https://github.com/DIAGNijmegen/AbdomenMRUS-pca-surveillance/blob/dfd889da23d2cfb3a60e0fbe476f44399c1378ee/Environment/Dicom2MHD/dicom_archive.py}{\underline{here}} and \href{https://github.com/DIAGNijmegen/AbdomenMRUS-pca-surveillance/blob/dfd889da23d2cfb3a60e0fbe476f44399c1378ee/Preprocessing/Convert-DICOM-archive.ipynb}{\underline{here}}  (requires DIAG access). My contributions: 
\begin{itemize}
    \item Identified additional \seriesDescription s
    \item Sped up pipeline $16\times$, reducing total preprocessing time from approx. 8 days to approx. 12 hours
    \item Wrote documentation for preprocessing pipeline
    \item Solved bug where scans became scrambled or blank
    \item Solved bug where the \seriesDescription s where matched incorrectly (affected approx. 50 scans) 
    \item Wrote verification of MHA archive (mainly to ensure studies are properly written to disk)
    \item Delivered MHA archive with approx. 5000 new visits
\end{itemize}

\begin{table}[]
\caption{Series descriptions identified for T2W, ADC and high b-value}
\begin{tabular}{@{}lll@{}}
\toprule
\textbf{Sequence} & \textbf{Series description}                          & \textbf{Frequency} \\ \midrule
T2W axial         & t2\_tse\_tra                                         & 9214                 \\
                  & t2\_tse\_tra\_snel                                   & 5941                 \\
                  & t2\_tse\_tra\_snel\_bij bewogen t2 tra               & 1184                 \\ \midrule
ADC               & ep2d\_diff\_tra\_ADC\_DFC                            & 8748                 \\
                  & \begin{tabular}[c]{@{}l@{}}diff tra b 50 500 800 WIP511b alle \\ spoelen\_ADC\end{tabular}      & 256                  \\
                  & ep2d\_diff\_tra\_orig\_ADC\_DFC                      & 47                   \\
                  & ep2d\_diff\_tra\_ADC                                 & 46                   \\
                  & diff tra b 50 500 800 WIP511E\_ADC                   & 32                   \\ \midrule
High b-value      & ep2d\_diff\_tra\_CALC\_BVAL\_DFC                     & 8748                 \\
                  & \begin{tabular}[c]{@{}l@{}}diff tra b 50 500 800 WIP511b alle \\ spoelenCALC\_BVAL\end{tabular} & 256                  \\
                  & ep2d\_diff\_tra\_orig\_CALC\_BVAL\_DFC               & 47                   \\
                  & ep2d\_diff\_tra\_CALC\_BVAL                          & 46                   \\
                  & diff tra b 50 500 800 WIP511ECALC\_BVAL              & 32                   \\ \midrule
T2W coronal       & t2\_tse\_cor                                         & 8747                 \\
                  & t2\_spc\_3D\_cor\_iso                                & 463                  \\ \midrule
T2W sagittal      & t2\_tse\_sag                                         & 9214                 \\ \midrule
Do NOT use        & resolve\_diff\_tra\_CALC\_BVAL                       & 248                  \\
                  & resolve\_diff\_tra\_ADC                              & 248                  \\
                  & resolve\_diff\_b50\_400\_800\_tra\_CALC\_BVAL        & 37                   \\
                  & resolve\_diff\_b50\_400\_800\_tra\_ADC               & 37                   \\ \bottomrule
\end{tabular}
\label{tab:MRI-sequences}
\end{table}

%%%%%%%%%%%%%%%%%%%%%%
%% RUMC annotations %%
%%%%%%%%%%%%%%%%%%%%%%
\subsubsection{Improving RUMC annotations}
\label{sec:improving-RUMC-annotations}
Annotations are one of the most important ingredients for training deep neural networks. During my internship I've worked on improving the annotations though combining different sources of information. Most notably, I've automatically split the majority of the PI-RADS $\geq 4$ annotations in separate PI-RADS 4 or 5 labels, and identified \percentageIncorrectAnnotationsIdentified\ cases with incorrect annotation (\percentageIncorrectAnnotationsIdentified\ of all annotations). 

Splitting the annotations in separate labels for PI-RADS 4 or 5 allows to train a machine learning model with improved risk-stratification, by assigning a higher risk to PI-RADS 5 than to PI-RADS 4. Split annotations also allow more fine-grained meta-analysis, and paved the way to also annotate the PI-RADS 3 lesions as a separate label. The automatic conversion script was able to confidently split 3,540/3,652 ($97\%$) cases, leaving 112 cases. These 112 remaining cases have been manually split by Ilse, meaning the annotation archive is now completely split into PI-RADS 4 and 5. 

% comment:22: Splitting csPCa annotations into PI-RADS 4 or 5
% comment:29: Dataset conversion

My contributions: 
\begin{itemize}
    \item Automatically split 3,540/3,652 ($97\%$) PI-RADS $\geq 4$ annotations in either PI-RADS 4 or 5
    \item Orchestrated several (small) annotation projects with Ilse 
    \item Set up GitHub archive for annotations, which makes adding and revising annotations transparent
    \item Identified \numIncorrectAnnotationsIdentified\ incorrect annotations (\percentageIncorrectAnnotationsIdentified\ of total). 
\end{itemize}

%% Corrected delineations %%
% See the overview in Development/2021-07-27-overview-revised-annotations

%%%%%%%%%%%%%%%%%%%
%% RUMC metadata %%
%%%%%%%%%%%%%%%%%%%
\subsubsection{Extracting metadata from reports}
\label{sec:extracting-RUMC-metadata}
The dataset from RUMC is derived from clinical practice over the span of seven years, resulting in a lot of useful information, but not necessarily in a structured format. Reliable metadata for all studies is important for most downstream analyses, so during my internship I've set out to extract metadata from the radiology and pathology reports. The benefit of radiology and pathology reports is that those are available across all years, but the drawback is that reports are free form text. 

Apart from extracting PI-RADS scores from radiology reports, I've also extracted: 
\begin{itemize}
    \item Gleason scores and biopsy dates from pathology reports
    \item PSA level, PSA density, prostate volume, prior treatment and prior Gleason scores from radiology reports
\end{itemize}

The extraction method for this metadata is similar to the PI-RADS extraction described in \Cref{sec:automatic_finding_extraction}, albeit a bit simpler. Code can be found \href{https://github.com/DIAGNijmegen/AbdomenMRUS-pca-surveillance/blob/dfd889da23d2cfb3a60e0fbe476f44399c1378ee/Preprocessing/Enrich-Metadata.ipynb}{\underline{here}} (requires DIAG access). 

\input{figures/STARD-RUMC}
% comment:15
% comment:23
% comment:36: Automatic extraction of PI-RADS scores from radiology reports

%%%%%%%%%%%%%%%%%%%%%%%%%%%%%
%% RUMC exclusion criteria %%
%%%%%%%%%%%%%%%%%%%%%%%%%%%%%
\subsubsection{Exclusion criteria RUMC}
\label{sec:exclusion-criteria-RUMC}
Studies with treatment or a positive biopsy (Gleason score $\geq 3+4$) prior to the MRI scan are excluded, as well as studies with bad MRI scan quality and studies from patients who opted out. 
To identify studies with prior treatment, I started with the list of treatments used by Matin, and extended that list by looking for additional treatments in the radiology reports. 
The list of treatments can be found in \Cref{tab:excluded-treatments}. 
I also excluded follow-up studies, even if the subsequent report didn't repeat the prior treatment. 
The improved pipelin resulted in identifying an additional \additionalTreatmentsFound\ studies with prior treatment (\additionalTreatmentsFoundPercentage\ more). 

Further documentation, details and lists of excluded studies can be found \href{https://github.com/DIAGNijmegen/AbdomenMRUS-pca-surveillance/blob/dfd889da23d2cfb3a60e0fbe476f44399c1378ee/Environment/config/exclusion_criteria.py}{\underline{here}} (requires DIAG access). The STARD diagram showing the number of studies included and excluded in this work is shown in \Cref{fig:STARD-RUMC}. 
% comment:19
% comment:20
% comment:24: Exclusion criteria: prior treatment and image artifacts

\begin{table}[]
\caption{Excluded treatments}
\begin{tabular}{@{}lll@{}}
\toprule
\textbf{Previously matched treatments}      & \textbf{Additional treatments} &  \\ \midrule
RALP                                        & TUR                            &  \\
Robotic-assisted laparoscopic prostatectomy & laser focale                   &  \\
laparoscopic                                & TULSA                          &  \\
radiotherapie                               & prostectomie                   &  \\
radiation                                   & focale behandeling             &  \\
radiotherapy                                & MRI laser behandeling          &  \\
HIFU                                        & bestraling                     &  \\
prostectomy                                 & hemi-ablatie                   &  \\
TURP                                        & ablatie                        &  \\
resection                                   & laserablatie                   &  \\
cryo                                        & anteriorresectie               &  \\
prostatectomie                              & sigmoidresectie                &  \\
brachytherapie                              & Green light laser              &  \\
therapie                                    & TURT                           &  \\
resectie                                    & chemotherapie                  &  \\
RRP                                         & LHRH                           &  \\
radicale prostatectomy                      &                                &  \\
prostatectomy                               &                                &  \\
EBRT                                        &                                &  \\
radiation therapy                           &                                &  \\
chemoradiatie                               &                                &  \\
na de chirurgie                             &                                &  \\
chirurgie                                   &                                &  \\
Hormonen                                    &                                &  \\
TURS                                        &                                &  \\ \bottomrule
\end{tabular}
\label{tab:excluded-treatments}
\end{table}

%%%%%%%%%%
%% UMCG %%
%%%%%%%%%%
\subsubsection{UMCG dataset}
\label{sec:preprocessing-UMCG-dataset}
The dataset from UMCG remained unused in my project, but I did prepare it. This involved collaborating with Jeroen and Christian to receive additional metadata, documentation and understanding their naming scheme. Furthermore, I extended the preprocessing pipeline described in \Cref{sec:preprocessing-RUMC-visits} to harmonise the datasets from UMCG and RUMC. The prepared dataset and documentation can be found at \verb!Chansey::pelvis/data/prostate-MRI/umcg/!. Code can be found \href{https://github.com/DIAGNijmegen/AbdomenMRUS-pca-surveillance/blob/dfd889da23d2cfb3a60e0fbe476f44399c1378ee/Preprocessing/Convert-RUMC-Annotations.ipynb}{\underline{here}} and \href{https://github.com/DIAGNijmegen/AbdomenMRUS-pca-surveillance/blob/dfd889da23d2cfb3a60e0fbe476f44399c1378ee/Preprocessing/Convert-UMCG-archive.ipynb}{\underline{here}} (requires DIAG access). 

Visits in our internal RUMC dataset are identified by a unique patient identifier and a unique study identifier. Using these two identifiers, it is straightforward to identify which studies belong to the same patient, and new visits can be added to the archive without affecting the naming scheme of existing visits. A similar naming scheme can be constructed for the UMCG dataset using their markdatasheet. 

\newcommand\patientID{\texttt{anon\_id}}
\newcommand\visitNum{\texttt{ret\_pat\_number}}
\newcommand\redcapID{\texttt{redcap\_id}}
\newcommand\studyID{\texttt{[redcap\_id]-[ret\_pat\_number]}}
Visits in the external UMCG dataset can be uniquely identified using the \redcapID\ (1 to 965) and \visitNum\ (empty for first visit, 1 for second visit and 2 for third visit), and patients can be uniquely identified using the \patientID\ (e.g., M-001 or U-001). To harmonise the naming scheme with the RUMC dataset, the \redcapID\ and \visitNum\ are combined to a unique study identifier as \studyID, where an empty \visitNum\ is replaced by a zero.

% patient id: M-ddd or U-ddd, with ddd a three-digit number. 
% visit num: empty for first visit, 1 for second, 2 for third, ...
% redcap id: identifier for (a sequence of) visits of a patients

The UMCG dataset consists of MRI examinations from UMCG, Martini Ziekenhuis and peripheral hospitals throughout the province of Groningen. Studies from UMCG or Martini have \texttt{mri\_location\_1 == 1}, while studies from peripheral hospitals have \texttt{mri\_location\_1 == 2}, with the specific peripheral hospital described in \texttt{mri\_location\_2}. Studies from peripheral hospitals have large variance in acquisition parameters, so only including studies from UMCG or Martini may be recommended. 

Further study selection criteria are prior treatment, prior positive biopsies and bad scan quality. 
Prior treatment was an exclusion criteria for the UMCG dataset, so none of the studies we received should have prior treatment. Bad scan quality wasn't an explicit exclusion criterion, but scans that are of insufficient quality for interpretation are usually repeated, and if all went well we only received good scans. To exclude studies with previously confirmed prostate cancer we received an updated markdatasheet, with prior Gleason scores described in \texttt{prev\_tar\_gleas1}, \texttt{prev\_tar\_gleas2}, \texttt{prev\_trus\_g1} and \texttt{prev\_trus\_g2}. 

Although the UMCG dataset is of very high quality, it did contain several naming inconsistencies in its files, likely caused by manual typing errors. To resolve these inconsistencies in a transparent manner, Anindo and I created a \href{https://github.com/DIAGNijmegen/prostateMR_archive_umcg}{\underline{repository}} for the annotations and corrected the typing mistakes.
