# Supplementary material for: Annotation-efficient cancer detection with report-guided lesion annotation for deep learning-based prostate cancer detection in bpMRI
Source: arXiv:2112.05151 source file (2022-02-19)
Supplement: Supplementary file 12 [file c-active-surveillance.tex]

\subsection{Active Surveillance}
Active Surveillance within prostate cancer management is an interesting and important direction to improve patient care. Working on deep learning solutions for Active Surveillance patients has taught me a lot, but did not result in concrete results. This lack of results was mainly caused by insufficient clinical motivation for the desired outcome. While existing Active Surveillance programs have shown excellent low prostate cancer mortality \citep{welty2015extended, selvadurai2013medium, klotz2015long, tosoian2015intermediate, bokhorst2016decade}, it is still relatively new. As a result, there is no clear target objective that a deep learning solution should aim for. 

Several options for target objectives exist: 
\begin{enumerate}
    \item Progression from Gleason grade group $\leq 1$ to Gleason grade group $\geq 2$
    \item Progression of PI-RADS score
    \item Identify new or vanished lesions
    \item Change of mean/min/std. ADC values within lesion mask
    \item Progression of lesion volume
\end{enumerate}

Unfortunately, all targets have limitations. Only few patients undergo multiple biopsies (1); PI-RADS scores suffer from large inter- and intra-reader variability, which is amplify when deriving change (2 \& 3); contours of lesions are often ill-defined, resulting in unstable statistics and volume (4 \& 5). 

The interested reader is encouraged to contact me (\href{mailto:Joeran.Bosma@radboudumc.nl}{Joeran.Bosma@radboudumc.nl}) for further discussions about Active Surveillance within prostate cancer management, and/or read the literature review I wrote on the deep learning side of it (\href{https://bosma.co/Bosma2021deep.pdf}{bosma.co/Bosma2021deep.pdf}. 

% Literature review: bosma.co/Bosma2021deep.pdf
