# Supplementary material for: Annotation-efficient cancer detection with report-guided lesion annotation for deep learning-based prostate cancer detection in bpMRI
Source: arXiv:2112.05151 source file (2022-02-19)
Supplement: Supplementary file 13 [file d-image-registration.tex]

\subsection{Image registration}
Image registration is a technique that can align medical scans that are similar but not exactly the same, which can be extremely helpful for a baseline and follow-up scan. 
An example is shown in \Cref{fig:registration-example}, where the first and third panel show the baseline and follow-up visits, and the second panel shows the baseline scan aligned to the follow-up scan. To align the baseline scan, it is moved `up' (towards anterior) and `pulled out of the page' (towards base), resulting in an aligned prostate. 

During my investigation of image registration for prostate MRI, I learned three practical lessons which I'd like to share:
\begin{enumerate}
    \item Normalise your scans before registration. Similar to deep learning, an image registration algorithm uses gradient ascent to optimise a similarity metric, and a registration can completely fail if those gradients are e.g. 1000 times higher than expected. 
    \item Registering the prostate segmentation masks, rather than the original scans, gives the most robust registration. A fine-grained registration of the original scans can then be compared to the robust registration, to spot cases where the fine-grained registration completely failed. 
    \item The structural similarity index metric (SSIM) is the metric that corresponds best with the true displacement, as shown by my brother \citep{bosma2021quantitative}. 
\end{enumerate}

% Image registration is difficult to quantitatively evaluate, 
% When I was working on Active Surveillance within prostate cancer diagnosis, I investigated image registration

\input{figures/registration-example}
