# Supplementary material for: Annotation-efficient cancer detection with report-guided lesion annotation for deep learning-based prostate cancer detection in bpMRI
Source: arXiv:2112.05151 source file (2022-02-19)
Supplement: Supplementary file 14 [file e-dynamic-threshold-pipeline.tex]

\subsection{Dynamic candidate extraction from softmax predictions}
When I started my internship, the method to extract lesion candidates from a model's softmax prediction involved a static threshold. Below this threshold, all model predictions were set to zero, and the remaining `islands' would then be the lesion candidates. This threshold was static across all samples, even though different models and even different datasets have different optimal thresholds. Other than tuning the static threshold for each model and dataset, there was no way to deduce a proper threshold. 

To circumvent the limitation of a static candidate extraction, I proposed a sample-dependent `dynamic' candidate extraction. This candidate extraction pipeline should extract `blobs' from the softmax prediction in a scale-free manner. The method I proposed defines a lesion candidate by selecting the most confident voxel as the `peak' and extending the lesion candidate until $40\%$ of its peak confidence. To extract multiple lesion candidates, this process is repeated. See \Cref{fig:dynamic-threshold-pipeline-large} for an example. 

\input{figures/dynamic-threshold-pipeline-large}

To validate the dynamic extraction of lesion candidates, I compared model performance obtained using the dynamic extraction pipeline against a range of static thresholds, as well as a sample-dependent threshold obtained using Otsu's method and a sample-dependent threshold defined as $40\%$ of the sample's peak. Please note that the latter method is different from the dynamic pipeline because it applies a single threshold and extracts all subsequent `islands', instead of the iterative approach of the dynamic extraction, and is termed `dynamic-fast'. Results for my baseline models (at the time of investigating the dynamic lesion candidate extraction), with 5-fold cross-validation and 5 restarts are shown in \Cref{fig:dynamic-threshold-FROC-performance}. Results for my models trained on automatic annotations (which used soft labels at the time), with 5-fold cross-validation and 3 restarts are shown in \Cref{fig:dynamic-threshold-FROC-performance-AVA}. The dynamic lesion candidate extraction either performs on par or outperforms the best static threshold, across all metrics. Most importantly, the dynamic extraction did not require any tuning, while the static pipeline has different optimal thresholds across metrics and models.

\input{figures/dynamic-threshold-FROC-performance}
\input{figures/dynamic-threshold-FROC-performance-pseudo-labels}
